# Supplementary material for: Accelerating the force-coupling method for hydrodynamic interactions in periodic domains
Source: arXiv:2310.12651 source file (2024-03-04)
Supplement: Supplementary file 1 [file algorithm.tex]

\appendix

\section{CUDA parallisation}\label{apx:cuda}
We provide here the parallisation strategy for the Fast FCM algorithms stated in the above section.

Step.1-3: Assign one thread per particle to compute the hash value and to update the cell list. We used the linearly scaling and parallelised radix sort function in the CUDA $cub$ library to sort particles.

Step.4, 6: There are two main categories of particle-based gridding algorithm using CUDA programming, referred to as thread per particle (TPP) and block per particle (BPP). For TPP, each thread is assigned one particle and is responsible to bridge the particle to all correlated $ngd^3$ grid points. For BPP, each block is assigned one particle and each thread within the same bridges the particle to a single grid point. The advantage of adopting BPP is that it has enough shared memory to store the $3\cdot ngd$ kernel weights by separating the kernel in each dimension, which is accessible to all threads. We use atomic operation when performing spreading to avoid race condition when different particles are accessing the same grid points. For gathering, the kernel weighted grid velocity is first stored in the register memory of individual thread, and at the end a reduction operation is performed to sum the values from all threads to get the particle velocity. This replaces the expensive atomic operation, reducing the time for gathering operation to one third of that of spreading. The detailed discussions of BPP and TPP gridding algorithms can be found in \cite{RAUL}. We report here that BPP always outperforms TPP in our implementation and is our adopted algorithm.

Step.5: The parallelised CUDA cuFFT toolkit is used to perform FFT and IFFT. We assign one thread per grid point to compute the Fourier flow velocity on the grid.

Step.7: Each thread is assigned one particle to check the distance between other particles within the same or neighbouring cells, and apply correction to the positive pairs.
